# Supplementary material for: Renting Edge Computing Resources for Service Hosting
Source: arXiv:2207.14690 source file (2022-10-31)
Supplement: Supplementary file 1 [file simulations.tex]

\begin{figure}[H]
\centering
  \subfloat[ $\text{Poisson}(\lambda = 700)$]{%
   \includesvg[width=0.45\linewidth]{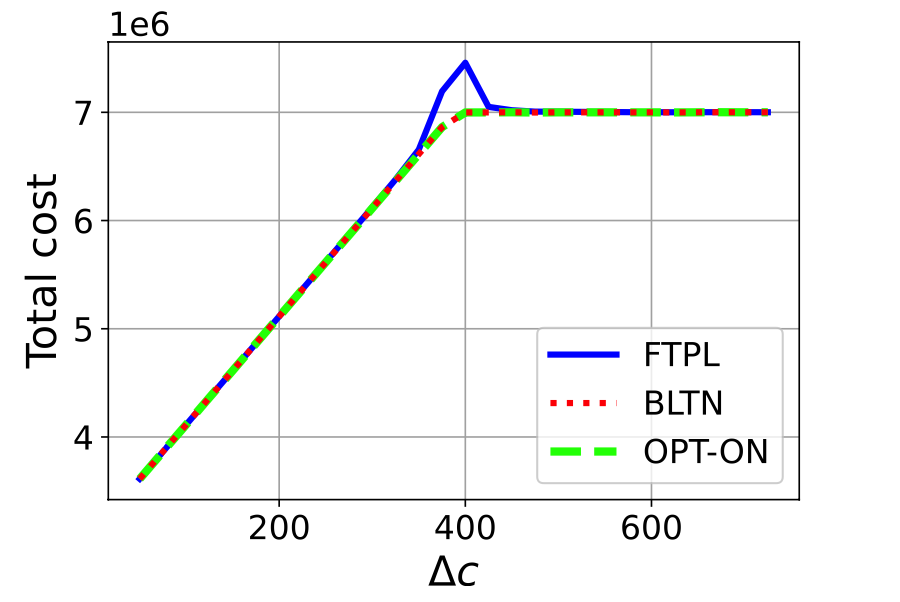}}
    \hspace{2pt}
    \subfloat[$GE(\lambda_H = 800,\lambda_L = 300)$]{%
   \includesvg[width=0.45\linewidth]{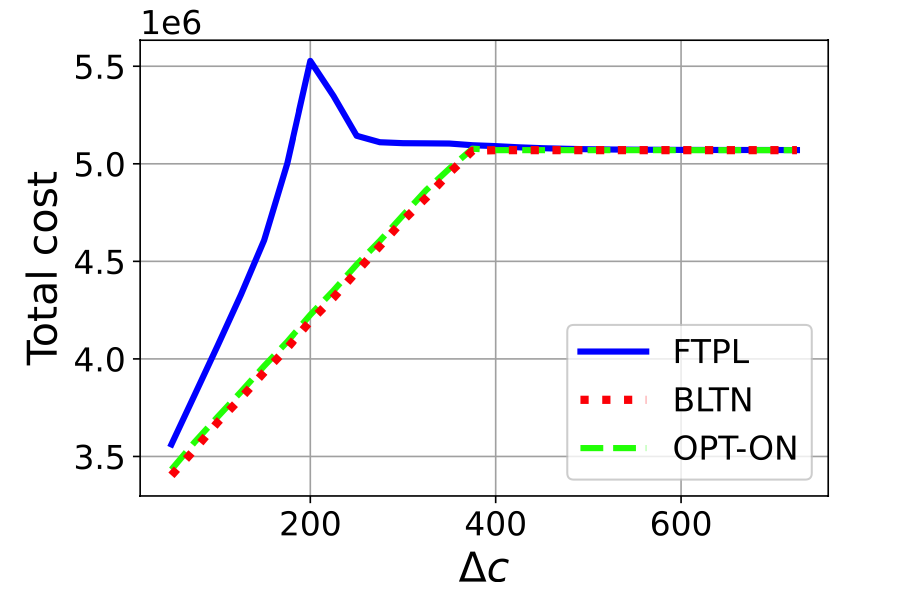}}
  \caption{Performance of various policies as a function of the difference in rent cost $\Delta c$.}
  \label{fig:c} 
\end{figure}

\begin{figure}
\centering
  \subfloat[ $\text{Poisson}(\lambda = 700)$]{%
   \includesvg[width=0.45\linewidth]{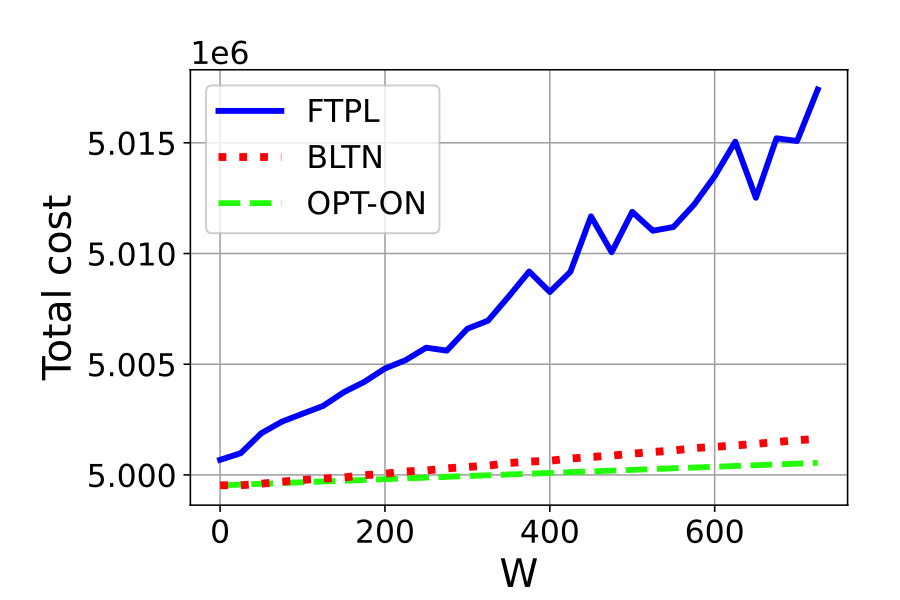}}
    \hspace{2pt}
    \subfloat[$GE(\lambda_H = 800,\lambda_L = 300)$]{%
   \includesvg[width=0.45\linewidth]{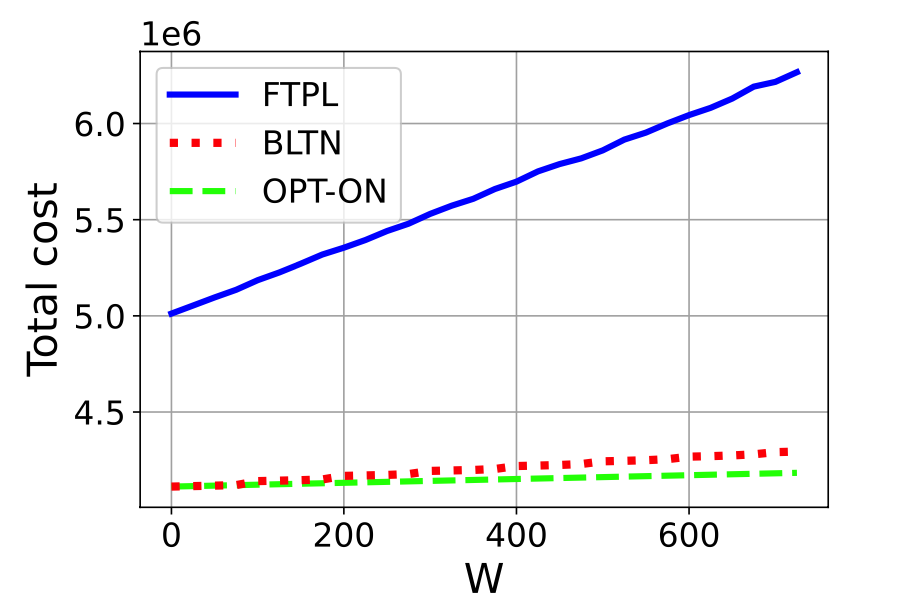}}
  \caption{Performance of various policies as a function of the switch cost $W = W_{HL} = W_{LH}$.}
  \label{fig:W} 
\end{figure}

% \begin{figure}
% \centering
%   \subfloat[ $\text{Poisson}(\lambda = 700)$]{%
%   \includesvg[width=0.47\linewidth]{plots/variation-lambda-64.svg}}
%     \hspace{2pt}
%     \subfloat[$GE(\lambda_H,\lambda_L = 300)$]{%
%   \includesvg[width=0.49\linewidth]{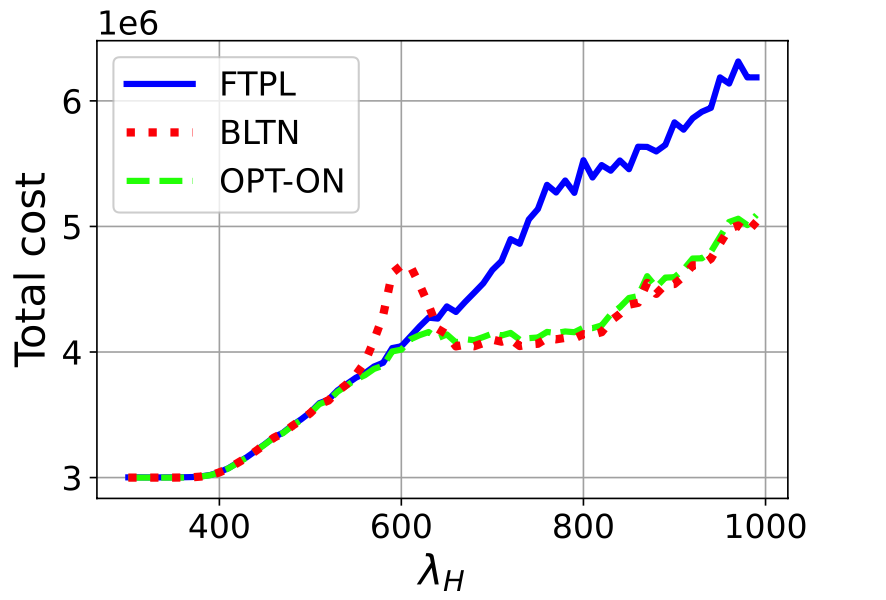}}
%   \caption{Variation with Poisson$(\lambda)$ arrivals}
%   \label{fig:lambda} 
% \end{figure}

% \begin{figure}
%     \centering
%     \includesvg[width = 0.9\columnwidth]{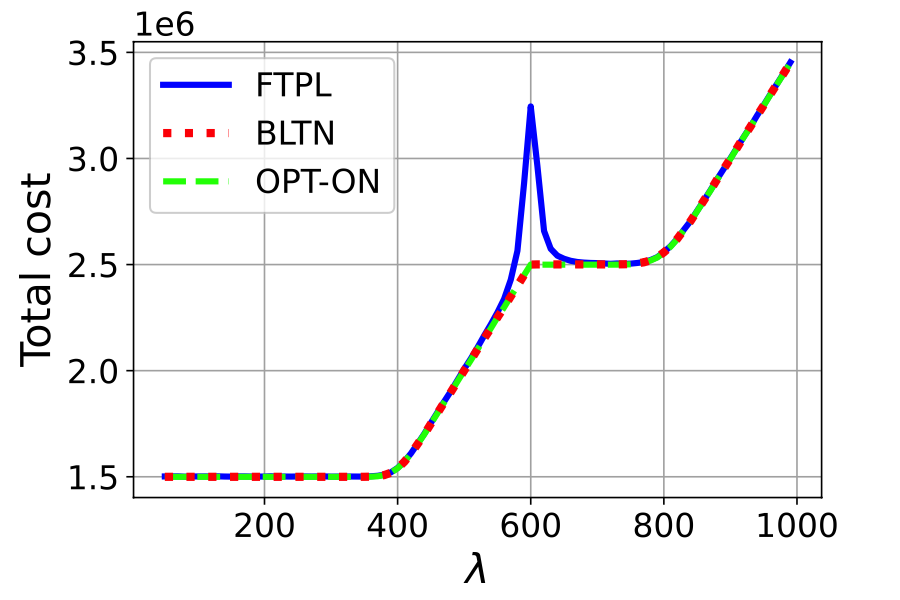}
%     \caption{Variation with Poisson$(\lambda)$ arrivals}
%     \label{fig:lambda}
% \end{figure}

%Significant differences are noticeable only under the Gilbert-Elliot like model and when $\Delta \kappa > \Delta c$ for Figures \ref{fig:c} and \ref{fig:W}.

\begin{figure}[H]
\centering
  \subfloat[ $\text{Poisson}(\lambda = 700)$]{%
   \includesvg[width=0.45\linewidth]{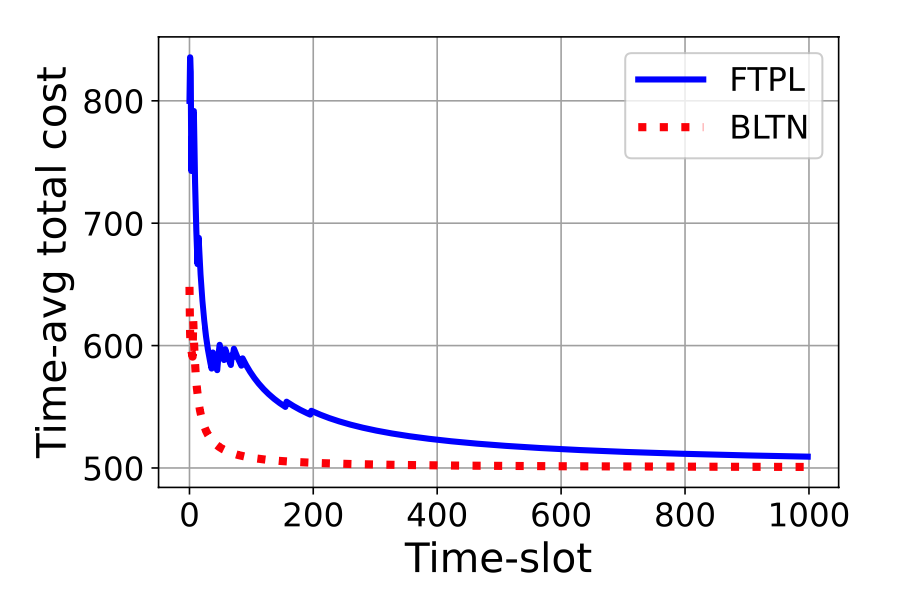}}
    \hspace{2pt}
    \subfloat[$GE(\lambda_H=800,\lambda_L = 300)$]{%
   \includesvg[width=0.45\linewidth]{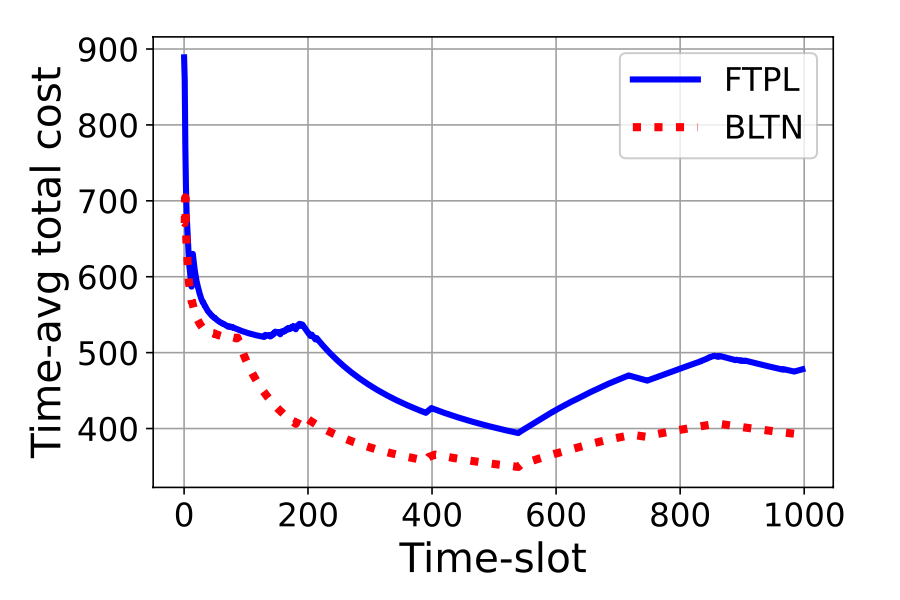}}
  \caption{Time averaged total cost}
  \label{fig:time-1000} 
\end{figure}

% \begin{figure}
%     \centering
%     \includesvg[width = 0.7\linewidth]{plots/variation-p-GE.svg}
%     \caption{Varying state transition probability \textit{p}}
%     \label{fig:time}
% \end{figure}
